# Supplementary material for: SEM-Net: Efficient Pixel Modelling for image inpainting with Spatially Enhanced SSM
Source: arXiv:2411.06318 source file (2024-11-10)
Supplement: Supplementary file 1 [file supp.pdf]

# Supplementary material - SEM-Net: Efficient Pixel Modelling for image inpainting with Spatially Enhanced SSM

Shuang Chen<sup>1</sup> Haozheng Zhang<sup>1</sup> Amir Atapour-Abarghouei<sup>1</sup> Hubert P. H. Shum<sup>1†</sup>

<sup>1</sup>{shuang.chen, haozheng.zhang, amir.atapour-abarghouei, hubert.shum}@durham.ac.uk

<sup>†</sup>Corresponding Author

## 1. Comparison of Sequential Modelling

We provide the illustration in Fig. 1 to showcase the difference between the proposed Snake Bi-Directional Modelling and simple sequential modelling. Tab. 1 showcases the quantitative results on CelebA-HQ in 40% – 60% mask ratio to compare with other optimizations of the SSM-based sequential modelling [1,5,6], demonstrating our superiority across all metrics.

Table 1. Comparison of different SSM-based modelling.

| Mask        | PSNR $\uparrow$ | SSIM $\uparrow$ | L <sub>1</sub> $\downarrow$ | FID $\downarrow$ | LPIPS $\downarrow$ |
|-------------|-----------------|-----------------|-----------------------------|------------------|--------------------|
| 2-D SSM [1] | 24.1153         | 0.7877          | 3.0950                      | 5.8556           | 0.1672             |
| VMamba [5]  | 24.1409         | 0.8031          | 2.9168                      | 5.9508           | 0.1739             |
| U-Mamba [6] | 24.2077         | 0.8119          | 2.7440                      | 5.6034           | 0.1466             |
| Ours        | <b>24.4805</b>  | <b>0.8240</b>   | <b>2.6389</b>               | <b>5.5972</b>    | <b>0.1368</b>      |

## 2. Experimental Details

**Image Inpainting** Except where specified differently, all experiments are conducted on a single Nvidia A100 GPU. We adopt the following set of parameters for our experiments: a batch size of 6 and a patch size of  $256 \times 256$ . We use Adam ( $\beta_1 = 0.9$ ,  $\beta_2 = 0.999$ ) optimizer with learning rate  $= 1e^{-4}$ . To achieve superior inpainting outcomes, we optimize our SEM-Net with the loss combination of  $\mathcal{L}_{total} = \lambda_1 \mathcal{L}_1 + \lambda_2 \mathcal{L}_{style} + \lambda_3 \mathcal{L}_{perc} + \lambda_4 \mathcal{L}_{adv}$ , where  $\lambda_1 = 1$ ,  $\lambda_2 = 250$ ,  $\lambda_3 = 0.1$ ,  $\lambda_4 = 0.001$ .  $\mathcal{L}_1$  is the pixel-wise reconstruction loss,  $\mathcal{L}_{style}$  is style loss,  $\mathcal{L}_{perc}$  is the perceptual loss, and  $\mathcal{L}_{adv}$  is the adversarial loss. We define the  $I_{gt}$  as the ground truth,  $I_{out}$  is the completed image,  $G$  is the SEM-Net and  $D$  is the discriminator. The formulation for each loss is shown below:

$$\mathcal{L}_{rec} = \mathbb{E} [\|I_{out} - I_{gt}\|_1], \quad (1)$$

$$\mathcal{L}_{perc} = \mathbb{E} \left[ \sum_i \|\phi_i(I_{out}) - \phi_i(I_{gt})\|_1 \right], \quad (2)$$

$$\mathcal{L}_{style} = \mathbb{E} \left[ \sum_i \|\psi_i(I_{out}) - \psi_i(I_{gt})\|_1 \right], \quad (3)$$

$$\mathcal{L}_{adv} = \min_G \max_D \mathbb{E}_{I_{gt}} [\log D(I_{gt})] + \mathbb{E}_{I_{out}} \log [1 - D(I_{out})], \quad (4)$$

where  $\phi_i(\cdot)$  indicates the activation map from the  $i$ -th pooling layer of VGG-16.  $\psi_i(\cdot) = \phi_i(\cdot)^T \phi_i(\cdot)$  denotes the Gram matrix. The loss combination of  $\mathcal{L}_{total} = \lambda_1 \mathcal{L}_1 + \lambda_2 \mathcal{L}_{style} + \lambda_3 \mathcal{L}_{perc} + \lambda_4 \mathcal{L}_{adv}$ , where  $\lambda_1 = 1$ ,  $\lambda_2 = 250$ ,  $\lambda_3 = 0.1$ ,  $\lambda_4 = 0.001$ .

**Image Deblurring** The image deblur task is formulated as  $I_{out} = I_{in} + SEM-Net(I_{in})$ , where  $I_{in}$  is the blurred image,  $I_{out}$  is the clear image. To train our deblurring model, we follow [2] to use a joint loss consisting of a reconstruction loss and a frequency loss. The formulation for each loss is shown below:

$$\mathcal{L}_{rec} = \mathbb{E} [\|I_{out} - I_{gt}\|_1], \quad (5)$$

$$\mathcal{L}_{frequency} = \mathbb{E} [\|F(I_{out}) - F(I_{gt})\|_1], \quad (6)$$

where  $F(\cdot)$  is the Fast Fourier transform. The total loss for image deblurring is  $L_{total} = L_{rec} + 0.1 \times L_{frequency}$ .

## 3. Additional Quantitative Results

Further ablation studies are showcased in the section. All models used in these experiments are trained for 30K iterations on CelebA-HQ dataset with a half-scaled SEM-Net. We also present the full tables for ablation study 3 and the comparison between our proposed SMB with other transformer-based methods 4 across all mask ratios.

### 3.1. Ablation study for Snake Bi-Directional Modelling (SBDM)

To further evaluate each design in the proposed Snake Bi-Directional Modelling (SBDM) module, we conduct the

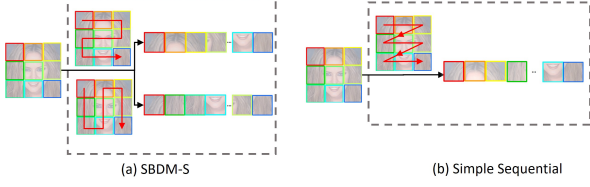

Figure 1. Comparison between (a) the proposed Snake Bi-Directional Modelling - Sequential (SBDM-S) and (b) the simple sequential approach. Our SBDM implicitly models bi-directional positional context by horizontally and vertically scanning the tokens, while the snake-shape design preserves the relations within adjacent tokens.

experiment by ablating each component. As shown in Tab. 4, *Bi-D* means horizontal and vertical direction modelling. The model without *Bi-D* only contains single horizontal direction modelling. *Snake* denotes the Snake-like Sequence Modelling. The model without *Snake* contains simple sequential modelling. We notice that the proposed snake-like design and bidirectional design overall improve the performance. An interesting observation is that at the largest mask ratio, individually integrating each of the two designs degrades the FID. But the FID at the largest mask ratio gets better when both snake-like design and bidirectional design are used together. This may indicate that when the damaged region is large and challenging, both complementary methods need to be used simultaneously to achieve better inpainting results without fully convergent training.

### 3.2. Importance of the Last Skip Connection

To preserve the detailed texture and structure feature from the first level of the encoder, we refrain from reducing the channel capacity after the last skip connection. The comparison of these two approaches (i.e., with reducing channel capacity and without reducing channel capacity via a  $1 \times 1$  convolution) is shown in Tab. 5.

## 4. More Qualitative Results

### 4.1. More Image Inpainting Comparisons

We showcase more qualitative image inpainting results on both CelebA-HQ and Places2 datasets in Fig. 2 and Fig. 3. From Fig. 2, we observe that SEM-Net successfully inpaints the masked eye by effectively capturing long-range dependencies from the visible eye, making the inpainted eye has a significantly more consistent shape and colour with finer-grained features. In Places2, SEM-Net generates fewer artefacts and more coherent structures, ensuring contextual consistency of image texture and structure.

### 4.2. Higher Resolution Visualisation

We provide higher resolution image inpainting results to examine the scalability and generalisability of SEM-Net trained on  $256 \times 256$  Places2 images in processing unseen images of large resolution ( $2560 \times 1920$  and  $1920 \times 2560$ ), which is showcased in Fig. 4 and 5. In our verification, SEM-Net is able to inpaint images with 2k+ resolutions without a significant loss in image quality or coherence.

### 4.3. More Image Motion Deblurring Comparisons

we showcase more qualitative image motion deblurring results on GoPro (Fig. 6) and HIDE (Fig. 7) datasets to further evaluate the image representation learning capability and generalisation ability of SEN-Net. Both figures demonstrate that our model recovers more structural details and is more sharper and visually closer to the groundtruth than other methods.

Table 2. Ablation studies of each component trained on CelebA-HQ [4].

| Net | Components |         |      |      |    | 0.01%-20%      |               |               |               |               | 20%-40%        |               |               |               |               | 40%-60%        |               |               |               |               |
|-----|------------|---------|------|------|----|----------------|---------------|---------------|---------------|---------------|----------------|---------------|---------------|---------------|---------------|----------------|---------------|---------------|---------------|---------------|
|     | MB         | FN [11] | SEFN | SBDM | PE | PSNR↑          | SSIM↑         | L1↓           | FID↓          | LPIPS↓        | PSNR↑          | SSIM↑         | L1↓           | FID↓          | LPIPS↓        | PSNR↑          | SSIM↑         | L1↓           | FID↓          | LPIPS↓        |
| (a) |            |         |      |      |    | 33.5812        | 0.9537        | 0.5385        | 1.4877        | 0.0513        | 25.8971        | 0.8527        | 1.9786        | 4.4025        | 0.1480        | 21.6134        | 0.7308        | 4.1254        | 8.1732        | 0.2464        |
| (b) | ✓          | ✓       |      |      |    | 33.7596        | 0.9604        | 0.5274        | 1.4660        | 0.0442        | 26.0679        | 0.8729        | 1.8220        | 4.3759        | 0.1261        | 21.7828        | 0.7587        | 3.9117        | 8.0742        | 0.2227        |
| (c) | ✓          |         | ✓    |      |    | 34.1085        | 0.9624        | 0.5059        | 1.4147        | 0.0420        | 26.3048        | 0.8755        | 1.7299        | 4.3664        | 0.1187        | 22.0510        | 0.7682        | 3.7649        | 7.9871        | 0.2132        |
| (d) | ✓          | ✓       |      | ✓    |    | 33.8899        | 0.9614        | 0.5151        | 1.4534        | 0.0415        | 26.2217        | 0.8767        | 1.7635        | 4.3674        | 0.1181        | 21.9064        | 0.7653        | 3.7679        | 8.0214        | 0.2102        |
| (e) | ✓          |         | ✓    | ✓    |    | 34.1184        | 0.9624        | 0.5043        | 1.4010        | 0.0408        | 26.3452        | 0.8776        | 1.7155        | 4.3559        | 0.1174        | 22.0926        | 0.7692        | 3.7634        | 7.9174        | 0.2091        |
| (f) | ✓          | ✓       |      | ✓    | ✓  | 33.9455        | 0.9616        | 0.5128        | 1.3751        | 0.0412        | 26.4037        | 0.8790        | 1.7303        | 4.3004        | 0.1193        | 22.1776        | 0.7708        | 3.6747        | 7.9125        | 0.2095        |
| (g) | ✓          |         | ✓    | ✓    | ✓  | <b>34.1437</b> | <b>0.9627</b> | <b>0.4986</b> | <b>1.3548</b> | <b>0.0403</b> | <b>26.4728</b> | <b>0.8808</b> | <b>1.6947</b> | <b>4.2718</b> | <b>0.1145</b> | <b>22.1780</b> | <b>0.7725</b> | <b>3.6274</b> | <b>7.8915</b> | <b>0.2038</b> |

Table 3. Comparison between our proposed SMB with transformer-based methods.

| Input Resolution | Model    | 0.01%-20%      |               |               |               |               | 20%-40%        |               |               |               |               | 40%-60%        |               |               |               |               |
|------------------|----------|----------------|---------------|---------------|---------------|---------------|----------------|---------------|---------------|---------------|---------------|----------------|---------------|---------------|---------------|---------------|
|                  |          | PSNR↑          | SSIM↑         | L1↓           | FID↓          | LPIPS↓        | PSNR↑          | SSIM↑         | L1↓           | FID↓          | LPIPS↓        | PSNR↑          | SSIM↑         | L1↓           | FID↓          | LPIPS↓        |
| 256*256          | CSA [11] | 33.5878        | 0.9595        | 0.5451        | 2.7514        | 0.0462        | 25.9348        | 0.8712        | 1.8644        | 5.1404        | 0.1300        | 21.5362        | 0.7543        | 4.0471        | 8.1652        | 0.2326        |
|                  | SSA [3]  | Out of memory  |               |               |               |               | Out of memory  |               |               |               |               | Out of memory  |               |               |               |               |
|                  | SMB      | <b>33.9455</b> | <b>0.9616</b> | <b>0.5128</b> | <b>1.3751</b> | <b>0.0431</b> | <b>26.4037</b> | <b>0.8790</b> | <b>1.7303</b> | <b>4.3004</b> | <b>0.1193</b> | <b>22.1776</b> | <b>0.7708</b> | <b>3.6747</b> | <b>7.9125</b> | <b>0.2095</b> |
| 64*64            | SSA [3]  | 32.0110        | 0.9308        | 0.7354        | 0.8345        | 0.0375        | 24.5320        | 0.7121        | 3.3047        | 2.8991        | 0.1035        | 20.1655        | 0.7265        | 5.2256        | 5.5547        | 0.1702        |
|                  | SMB      | <b>32.0218</b> | <b>0.9437</b> | <b>0.7120</b> | <b>0.8152</b> | <b>0.0351</b> | <b>24.6112</b> | <b>0.7214</b> | <b>3.1575</b> | <b>2.7503</b> | <b>0.1022</b> | <b>20.1716</b> | <b>0.7352</b> | <b>5.1332</b> | <b>5.3158</b> | <b>0.1617</b> |

Table 4. Ablation study of each component trained on CelebA-HQ [4].

| Net | Components |      |       |    |      | 0.01%-20%      |               |               |               |               | 20%-40%        |               |               |               |               | 40%-60%        |               |               |               |               |
|-----|------------|------|-------|----|------|----------------|---------------|---------------|---------------|---------------|----------------|---------------|---------------|---------------|---------------|----------------|---------------|---------------|---------------|---------------|
|     | MB         | Bi-D | Snake | PE | SEFN | PSNR↑          | SSIM↑         | L1↓           | FID↓          | LPIPS↓        | PSNR↑          | SSIM↑         | L1↓           | FID↓          | LPIPS↓        | PSNR↑          | SSIM↑         | L1↓           | FID↓          | LPIPS↓        |
| (a) | ✓          |      |       | ✓  | ✓    | 34.1114        | 0.9624        | 0.5046        | 1.4134        | 0.0418        | 26.3305        | 0.8769        | 1.7231        | 4.3533        | 0.1186        | 22.0760        | 0.7688        | 3.7643        | 7.9868        | 0.2125        |
| (b) | ✓          | ✓    |       | ✓  | ✓    | 34.1428        | 0.9625        | 0.5016        | 1.3560        | 0.0416        | 26.4725        | 0.8802        | 1.7078        | 4.2751        | 0.1178        | 22.1351        | 0.7715        | 3.6742        | 8.0395        | 0.2078        |
| (c) | ✓          |      | ✓     | ✓  | ✓    | 34.1172        | 0.9624        | 0.5040        | 1.3564        | 0.0419        | 26.4619        | 0.8793        | 1.7105        | 4.2830        | 0.1185        | 22.1720        | 0.7692        | 3.6890        | 8.0372        | 0.2108        |
| (e) | ✓          | ✓    | ✓     | ✓  | ✓    | <b>34.1437</b> | <b>0.9627</b> | <b>0.4986</b> | <b>1.3548</b> | <b>0.0403</b> | <b>26.4728</b> | <b>0.8808</b> | <b>1.6947</b> | <b>4.2718</b> | <b>0.1145</b> | <b>22.1780</b> | <b>0.7725</b> | <b>3.6274</b> | <b>7.8915</b> | <b>0.2038</b> |

Table 5. Ablation study of using  $1 \times 1$  convolution after the last skip connection.

| Model                        | 0.01%-20%      |               |               |               |               | 20%-40%        |               |               |               |               | 40%-60%        |               |               |               |               |
|------------------------------|----------------|---------------|---------------|---------------|---------------|----------------|---------------|---------------|---------------|---------------|----------------|---------------|---------------|---------------|---------------|
|                              | PSNR↑          | SSIM↑         | L1↓           | FID↓          | LPIPS↓        | PSNR↑          | SSIM↑         | L1↓           | FID↓          | LPIPS↓        | PSNR↑          | SSIM↑         | L1↓           | FID↓          | LPIPS↓        |
| w $1 \times 1$ conv          | 33.9158        | 0.9614        | 0.5060        | 1.4503        | 0.0414        | 26.2481        | 0.8753        | 1.7605        | 4.3794        | 0.1185        | 22.0311        | 0.7700        | 3.7580        | 8.0976        | 0.2184        |
| w/o $1 \times 1$ conv (ours) | <b>34.1437</b> | <b>0.9627</b> | <b>0.4986</b> | <b>1.3548</b> | <b>0.0403</b> | <b>26.4728</b> | <b>0.8808</b> | <b>1.6947</b> | <b>4.2718</b> | <b>0.1145</b> | <b>22.1780</b> | <b>0.7725</b> | <b>3.6274</b> | <b>7.8915</b> | <b>0.2038</b> |

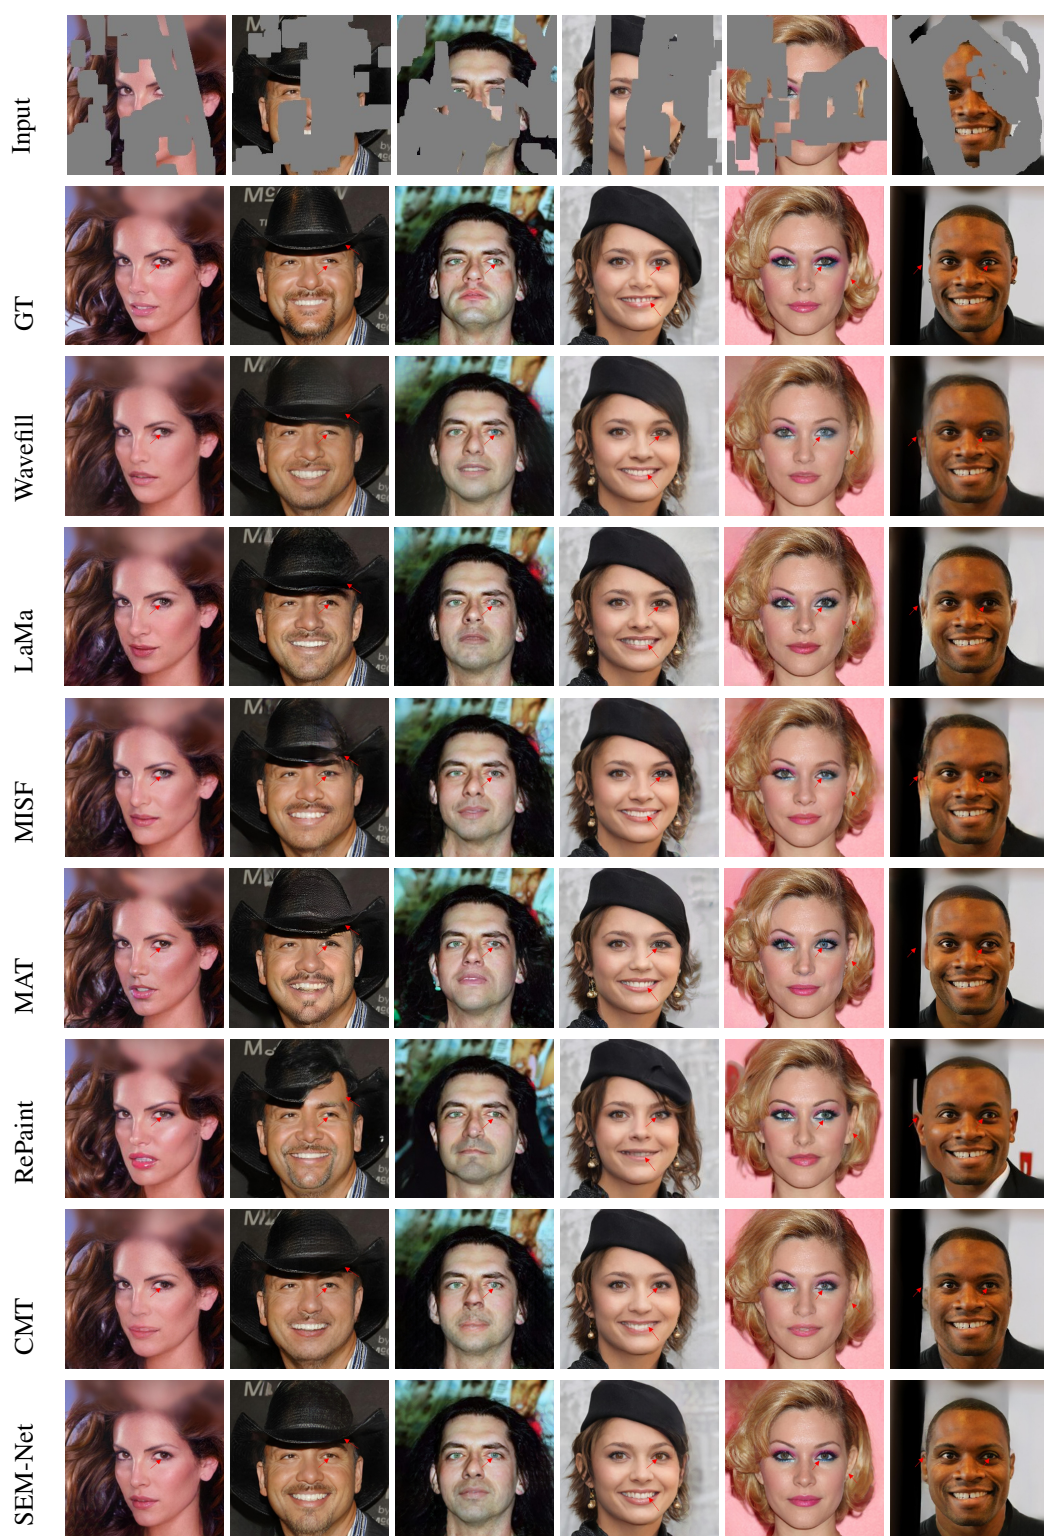

Figure 2. More visualisations ( $256 \times 256$ ) on the CelebA-HQ dataset. Please zoom in to see details.

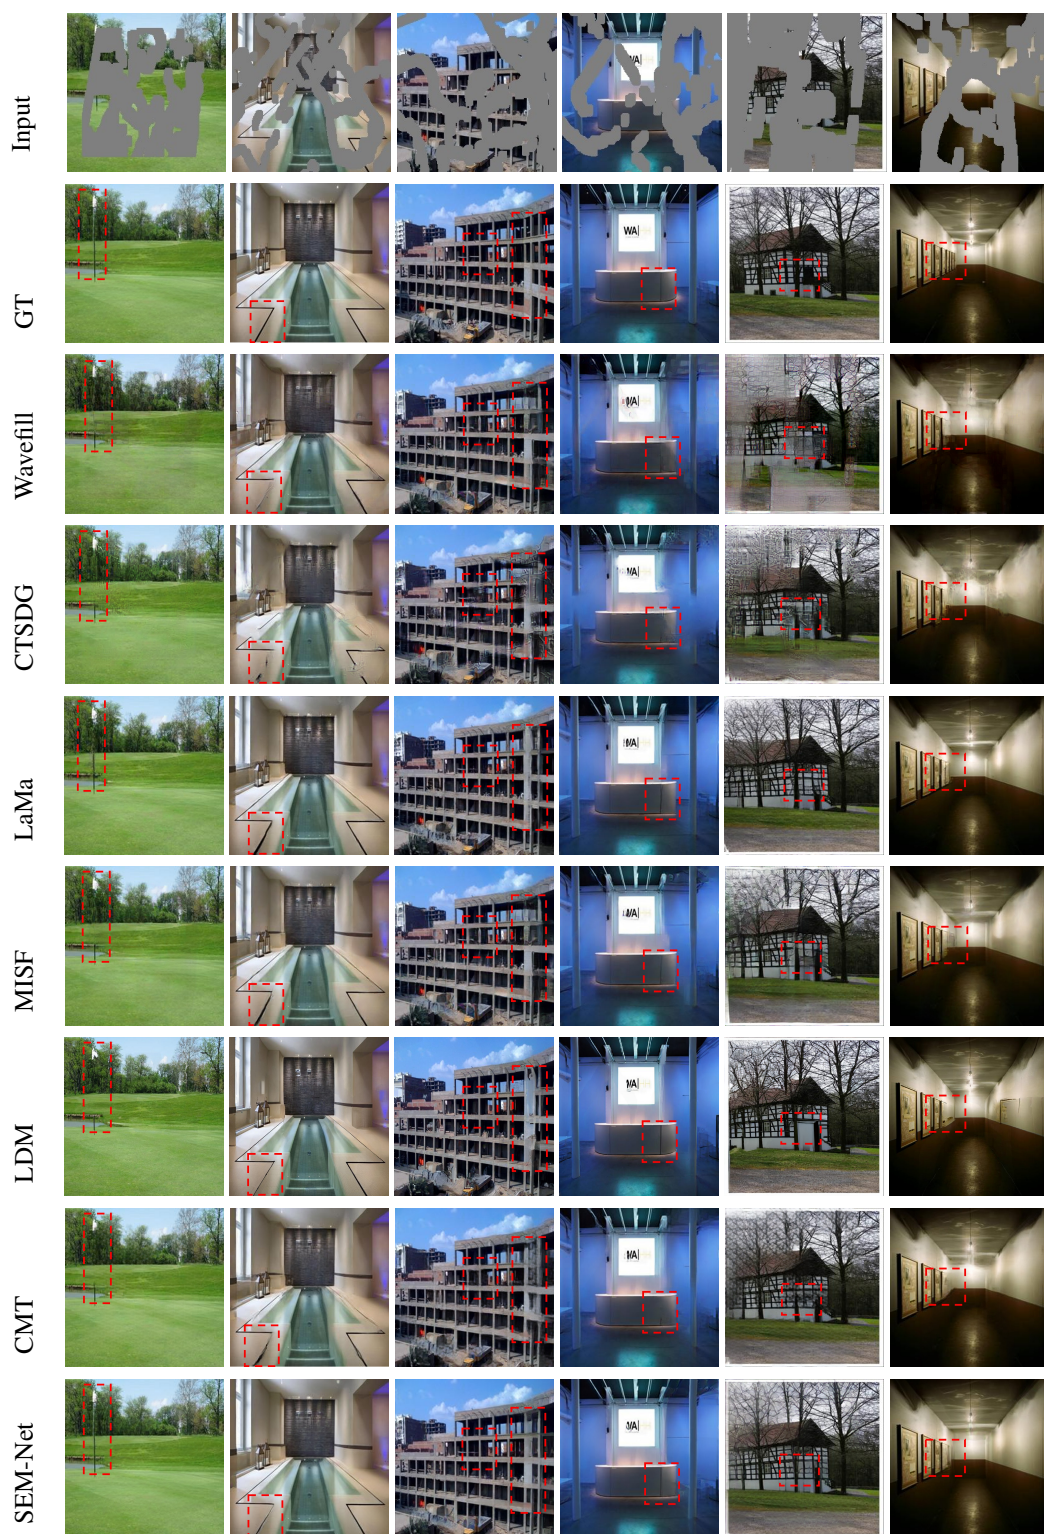

Figure 3. More visualisations ( $256 \times 256$ ) on the Places2 dataset. Please zoom in to see details.

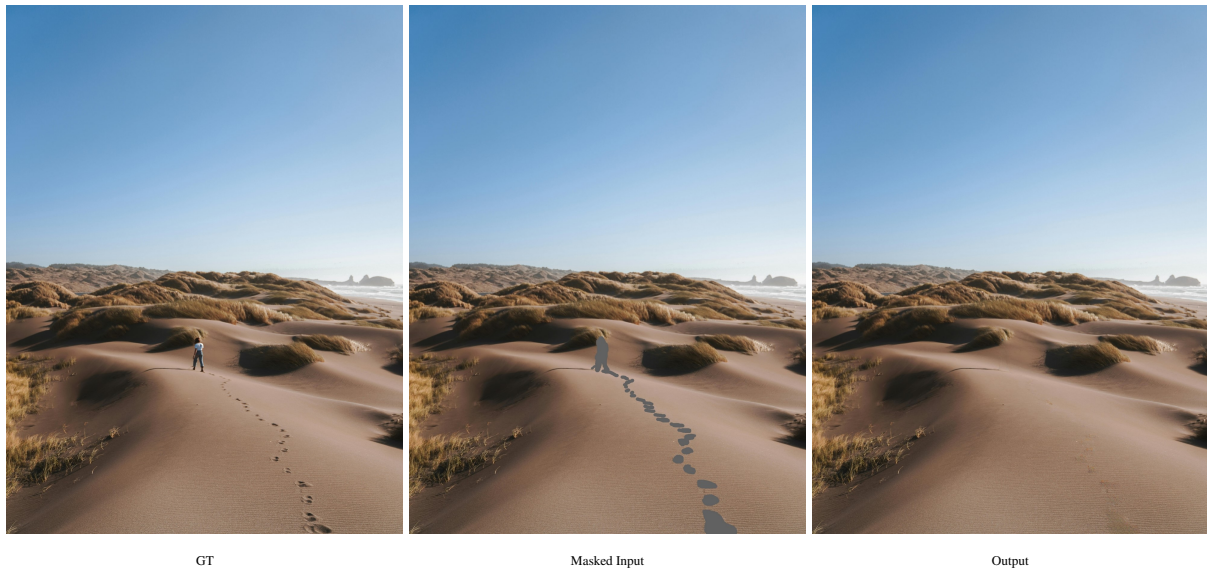

Figure 4. The example of generalisation to real-world high-resolution images of  $1920 \times 2560$ .

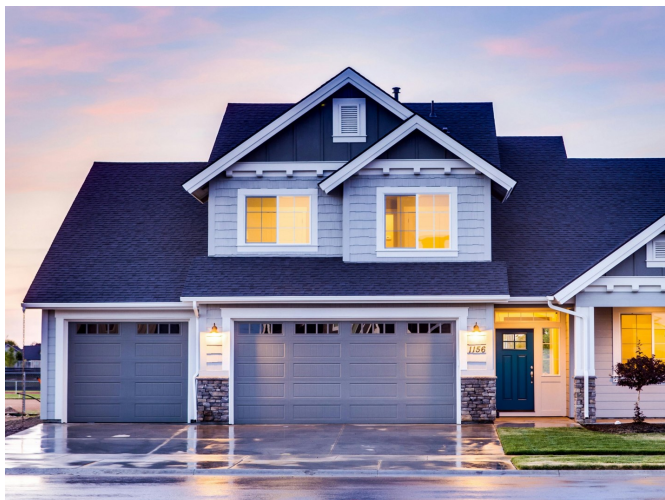

GT

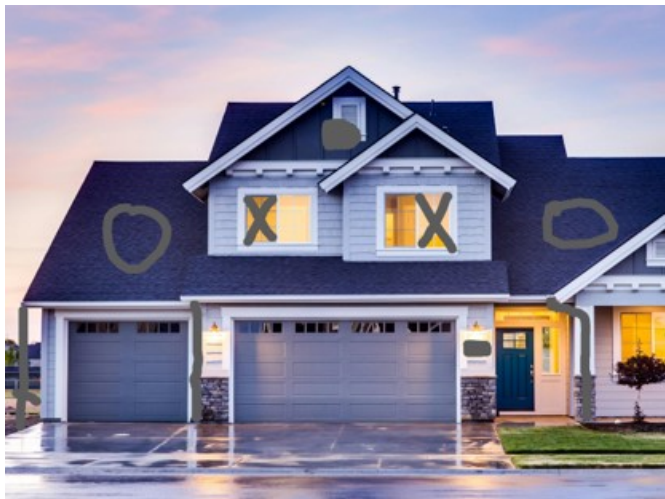

Masked Input

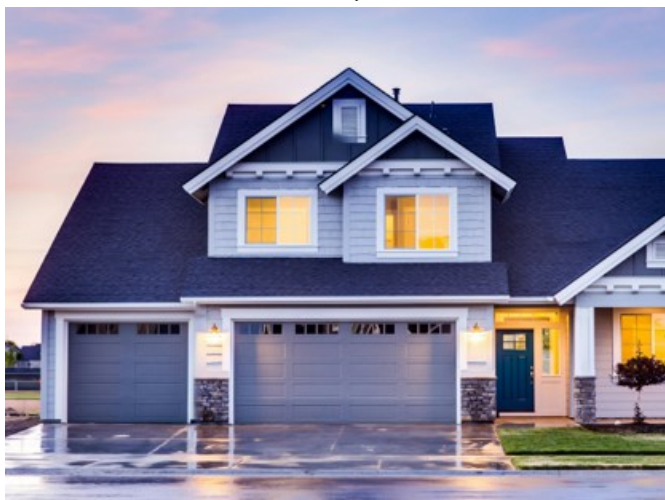

Output

Figure 5. The example of generalisation to real-world high-resolution images of  $2560 \times 1920$ .

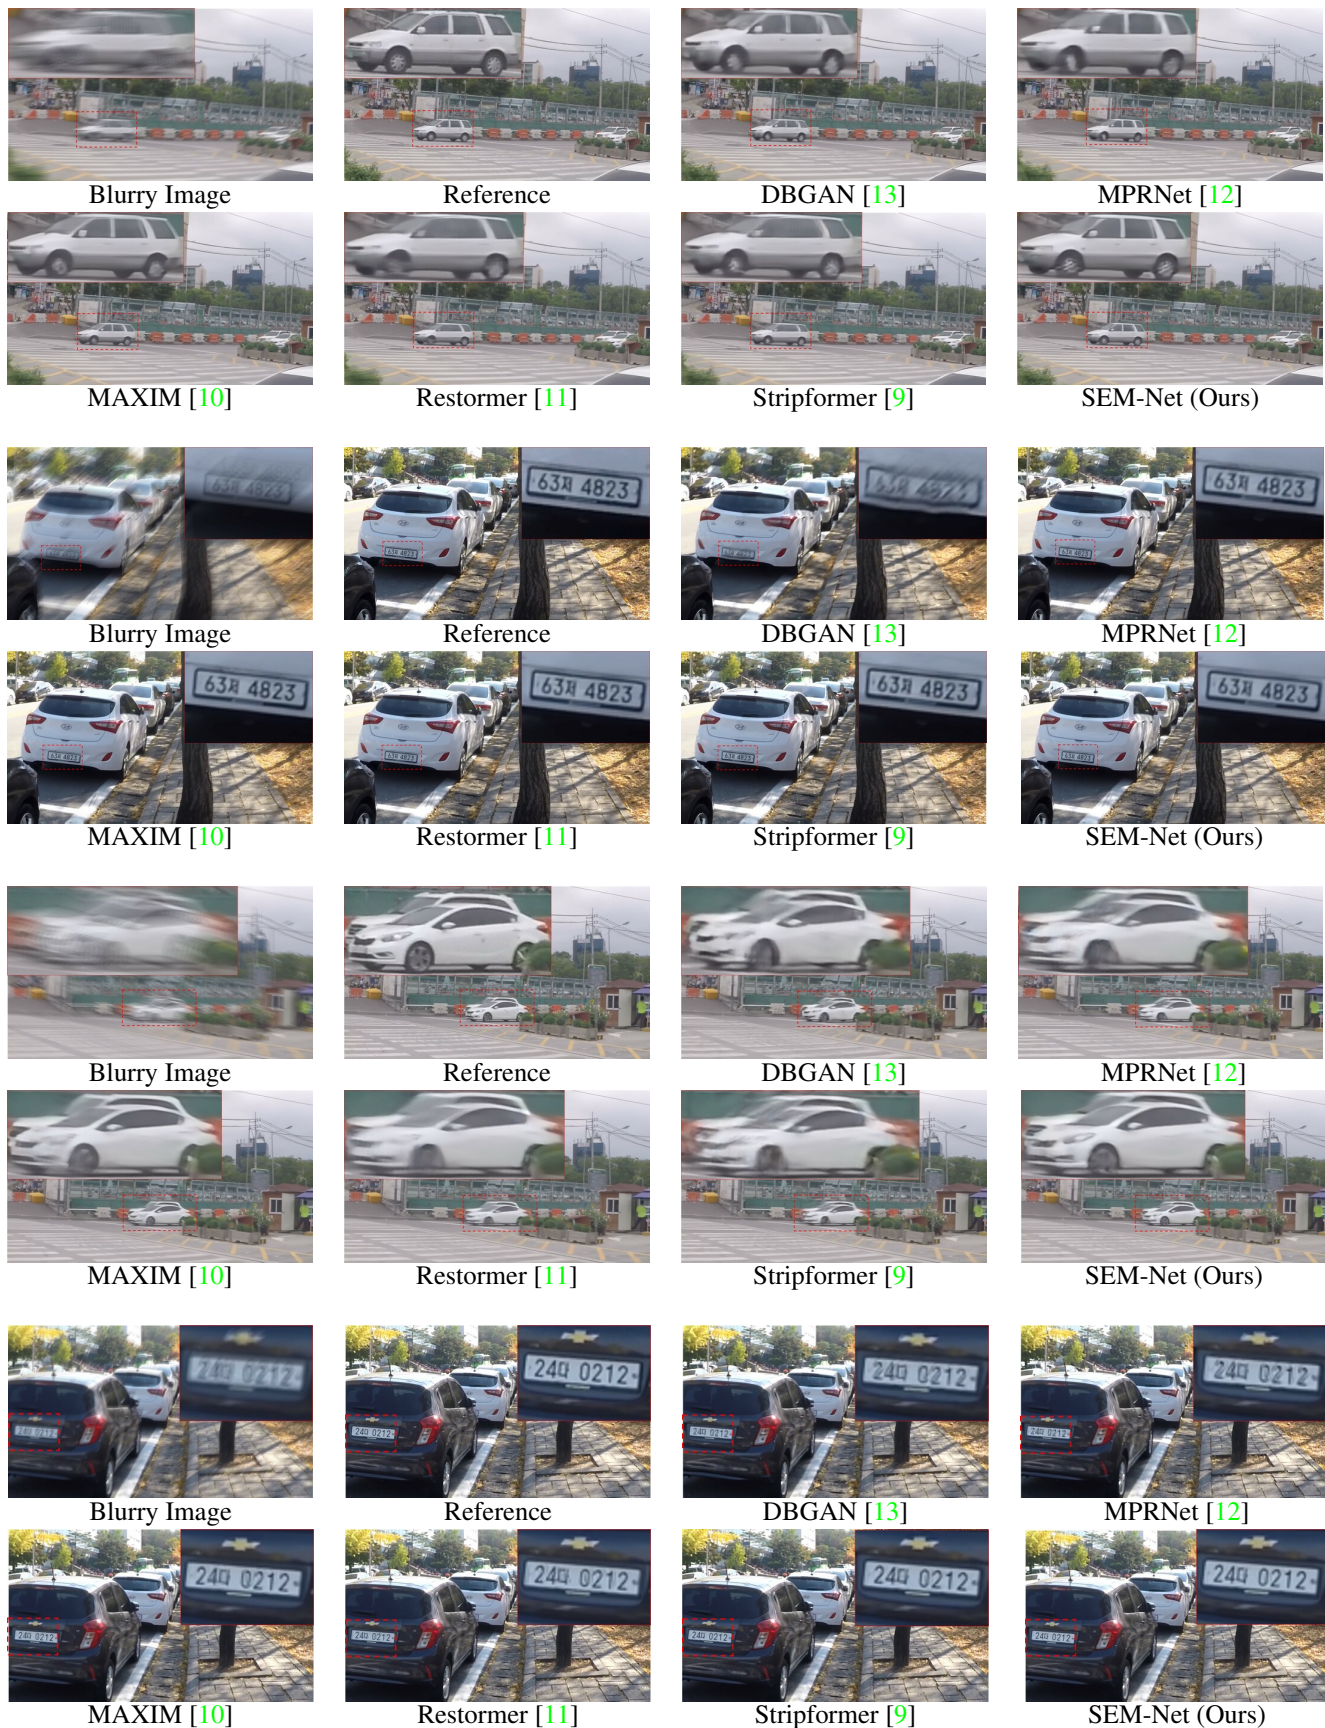

Figure 6. Image motion deblurring comparisons on GoPro [7]. Our method generates sharper results with higher visual fidelity.

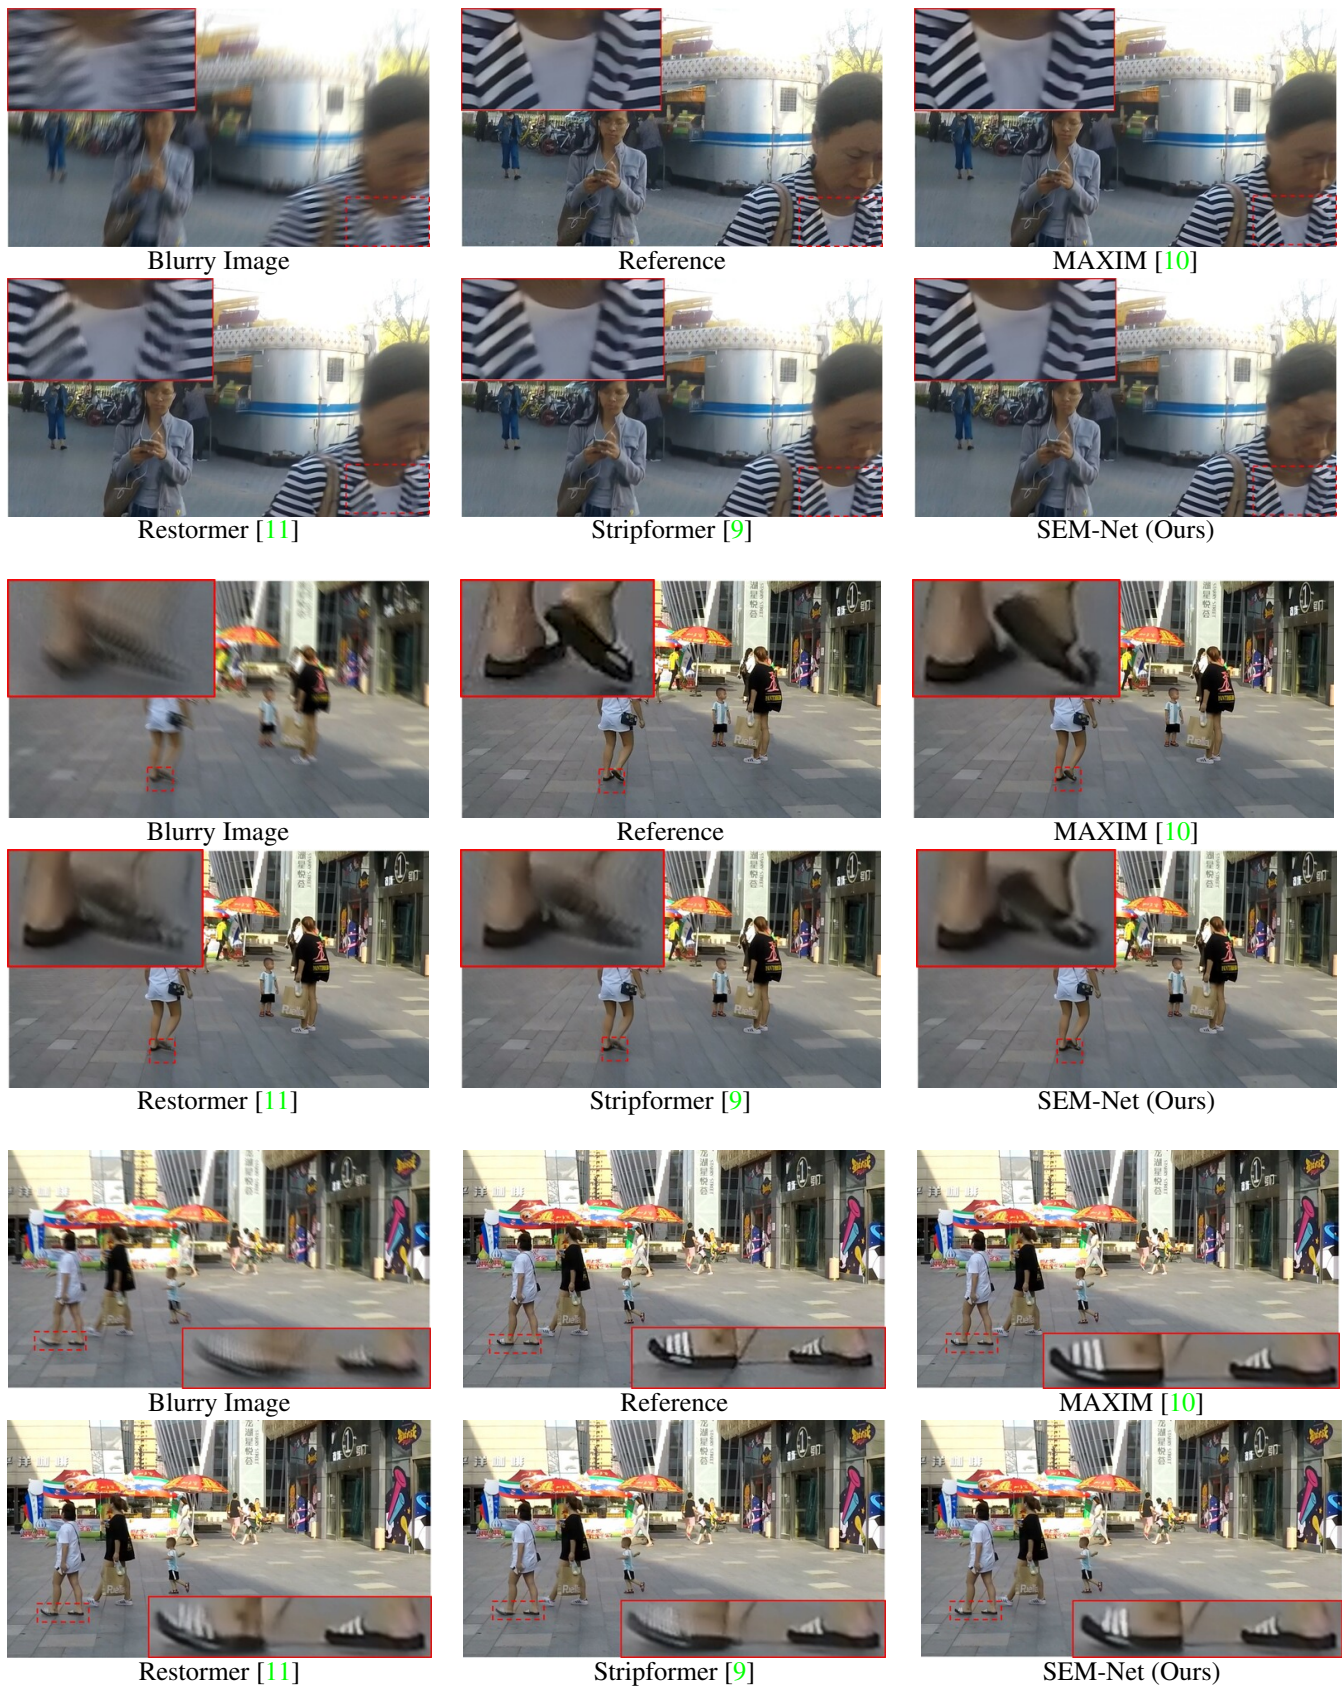

Figure 7. Image motion deblurring comparisons on HIDE [8]. Our methods generates sharper results with higher visual fidelity.

## References

- [1] Ethan Baron, Itamar Zimmerman, and Lior Wolf. 2-d ssm: A general spatial layer for visual transformers. *arXiv preprint arXiv:2306.06635*, 2023. 1
- [2] Yuning Cui, Yi Tao, Zhenshan Bing, Wenqi Ren, Xinwei Gao, Xiaochun Cao, Kai Huang, and Alois Knoll. Selective frequency network for image restoration. In *The Eleventh International Conference on Learning Representations*, 2022. 1
- [3] Alexey Dosovitskiy, Lucas Beyer, Alexander Kolesnikov, Dirk Weissenborn, Xiaohua Zhai, Thomas Unterthiner, Mostafa Dehghani, Matthias Minderer, Georg Heigold, Sylvain Gelly, et al. An image is worth 16x16 words: Transformers for image recognition at scale. *arXiv preprint arXiv:2010.11929*, 2020. 3
- [4] Tero Karras, Timo Aila, Samuli Laine, and Jaakko Lehtinen. Progressive growing of gans for improved quality, stability, and variation. *arXiv preprint arXiv:1710.10196*, 2017. 3
- [5] Yue Liu, Yunjie Tian, Yuzhong Zhao, Hongtian Yu, Lingxi Xie, Yaowei Wang, Qixiang Ye, and Yunfan Liu. Vmamba: Visual state space model. *arXiv preprint arXiv:2401.10166*, 2024. 1
- [6] Jun Ma, Feifei Li, and Bo Wang. U-mamba: Enhancing long-range dependency for biomedical image segmentation. *arXiv preprint arXiv:2401.04722*, 2024. 1
- [7] Seungjun Nah, Tae Hyun Kim, and Kyoung Mu Lee. Deep multi-scale convolutional neural network for dynamic scene deblurring. In *CVPR*, 2017. 8
- [8] Ziyi Shen, Wenguan Wang, Xiankai Lu, Jianbing Shen, Haibin Ling, Tingfa Xu, and Ling Shao. Human-aware motion deblurring. In *ICCV*, 2019. 9
- [9] Fu-Jen Tsai, Yan-Tsung Peng, Yen-Yu Lin, Chung-Chi Tsai, and Chia-Wen Lin. Stripformer: Strip transformer for fast image deblurring. In *European Conference on Computer Vision*, pages 146–162. Springer, 2022. 8, 9
- [10] Zhengzhong Tu, Hossein Talebi, Han Zhang, Feng Yang, Peyman Milanfar, Alan Bovik, and Yinxiao Li. Maxim: Multi-axis mlp for image processing. In *Proceedings of the IEEE/CVF Conference on Computer Vision and Pattern Recognition*, pages 5769–5780, 2022. 8, 9
- [11] Syed Waqas Zamir, Aditya Arora, Salman Khan, Munawar Hayat, Fahad Shahbaz Khan, and Ming-Hsuan Yang. Restormer: Efficient transformer for high-resolution image restoration. In *Proceedings of the IEEE/CVF conference on computer vision and pattern recognition*, pages 5728–5739, 2022. 3, 8, 9
- [12] Syed Waqas Zamir, Aditya Arora, Salman Khan, Munawar Hayat, Fahad Shahbaz Khan, Ming-Hsuan Yang, and Ling Shao. Multi-stage progressive image restoration. In *CVPR*, 2021. 8
- [13] Kaihao Zhang, Wenhan Luo, Yiran Zhong, Lin Ma, Bjorn Stenger, Wei Liu, and Hongdong Li. Deblurring by realistic blurring. In *CVPR*, 2020. 8
